# Supplementary material for: Magnetic excitations in the topological semimetal $\mathrm{YbMnSb}_2$
Source: arXiv:2302.07007 ancillary file (2023-02-14)
Supplement: Supplementary file 1 [file Magnetic_excitations_of_YbMnSb2_SUPPLEMENTAL.pdf]

# SUPPLEMENTAL MATERIAL
# Magnetic excitations of the topological semimetal $YbMnSb_2$

Siobhan M. Tobin,[1] Jian-Rui Soh,[2] Hao Su,[3] Andrea Piovano,[4] Anne Stunault,[4] J. Alberto Rodríguez-Velamazán,[4] Yanfeng Guo,[3,5] and Andrew T. Boothroyd[1]

[1] *Department of Physics, University of Oxford, Clarendon Laboratory, Oxford OX1 3PU, United Kingdom*
[2] *Institute of Physics, Ecole Polytechnique Fédérale de Lausanne (EPFL), CH-1015 Lausanne, Switzerland*
[3] *School of Physical Science and Technology, ShanghaiTech University, Shanghai 201210, China*
[4] *Institut Laue-Langevin, 6 rue Jules Horowitz, BP 156, 38042 Grenoble Cedex 9, France*
[5] *ShanghaiTech Laboratory for Topological Physics, ShanghaiTech University, Shanghai 201210, China*

(Dated: February 14, 2023)

## I. SAMPLE CHARACTERISATION

The flux-grown crystals of $YbMnSb_2$ came from the same batch as used in previous experiments [1]. The platelet crystals were individually examined via Laue x-ray diffraction and coaligned on an aluminium plate with the $c$ axis perpendicular to the plane of the plate. Crystals were affixed to the aluminium using CYTOP glue [2]. To estimate the mosaicity of the ensemble of 20 crystals combined, we stacked Laue images of individual crystals taken with the aluminium plate in a fixed orientation. The combined Laue image shows the patterns are translated slightly with respect to each other both horizontally and vertically, but the patterns hardly show any relative rotation. This implies the crystals are slightly misaligned in the $ac$ and $bc$ planes, most likely from the glue not drying completely flat. The mosaicity was estimated to be $\sim 3°$. The assembly of $YbMnSb_2$ crystals for inelastic neutron scattering on IN8 is shown in Fig. 1 together with the combined Laue figure.

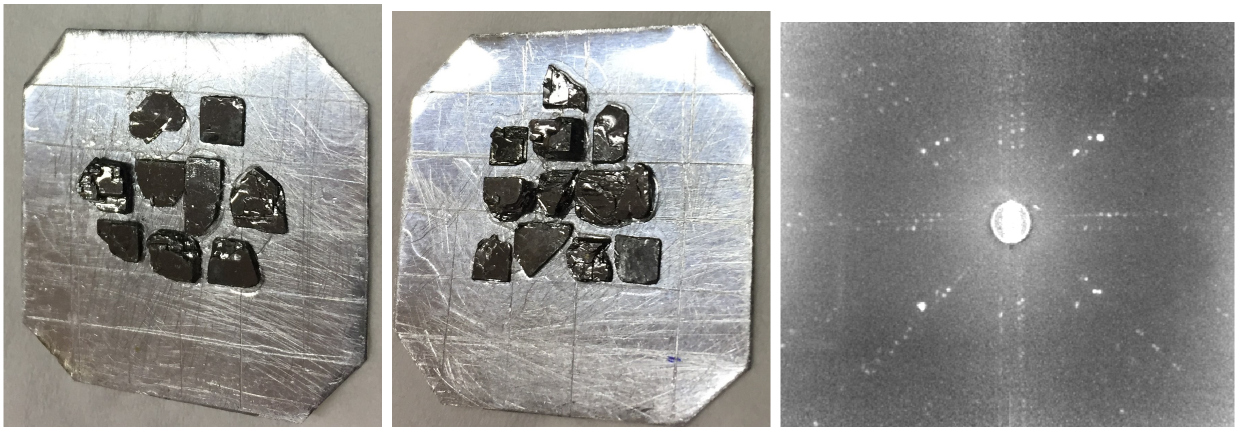

a) b) c)

FIG. 1. a) and b) both sides of sample of $YbMnSb_2$ prepared for inelastic neutron scattering experiment, c) combined x-ray Laue pattern of the assembly of crystals.

## II. INELASTIC NEUTRON SCATTERING DATA ANALYSIS

The inelastic neutron scattering data from the IN8 experiment contained both powder rings and 'spurions'. The IN8 Flatcone detector sweeps out arcs in reciprocal space, so the constant $\Delta E$ reciprocal space maps are best visualised as Voronoi diagrams, rather than a regular Cartesian grid. Our work presents both 'raw' and 'corrected' data. Here we describe the correction process, which was performed for each reciprocal space map at different $\Delta E$. Using NPlot [3] the spurions were removed by hand. The spin wave signal was also subtracted and the remaining background smoothed such that the background only depended on $Q$. This isotropic background was subtracted from the raw

data, and the ‘spurious’ data points were removed such that the size of Voronoi cells increased for regions containing spurions. This procedure generated the reciprocal space maps of ‘corrected’ data.

To enable faster data reduction, an interpolation was performed on the Voronoi diagrams to map the intensity to a regular Cartesian grid. Due to geometry of the IN8 instrument and the Flatcone array, the data are distorted slightly at higher $Q$ (for example, in the $h0l$ plane, the spin waves appear to curve away from lines of constant $h$). By symmetrising the data about Brillouin zone boundaries once the dimensionality of the data had been reduced by taking constant $\mathbf{Q}$ cuts, we accounted for this effect.

## III. INELASTIC NEUTRON SCATTERING DATA: CUTS ALONG Q WITH CONSTANT $\Delta E$

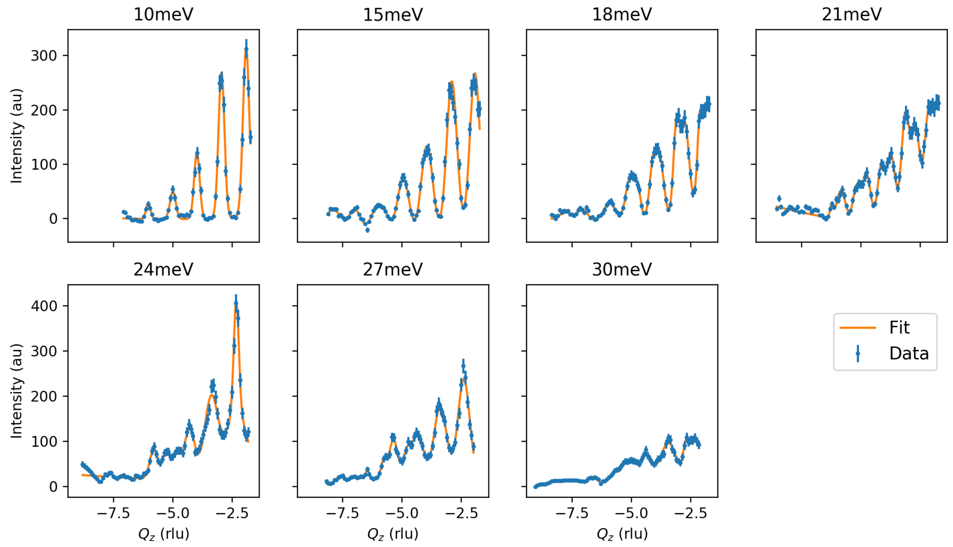


FIG. 2. One dimensional cuts along $\mathbf{Q} = (10l)$ at different $\Delta E$ from the data measured in the $h0l$ scattering plane. Fits are shown in orange.

[1] J.-R. Soh, S. M. Tobin, H. Su, I. Zivkovic, B. Ouladdiaf, A. Stunault, J. A. Rodríguez-Velamazán, K. Beauvois, Y. Guo, and A. T. Boothroyd, Magnetic structure of the topological semimetal ${\mathrm{YbMnSb}}_{2}$, Physical Review B **104**, L161103 (2021), publisher: American Physical Society.
[2] K. C. Rule, R. A. Mole, and D. Yu, Which glue to choose? A neutron scattering study of various adhesive materials and their effect on background scattering, Journal of Applied Crystallography **51**, 1766 (2018).
[3] P. Steffens, nplot (2019).

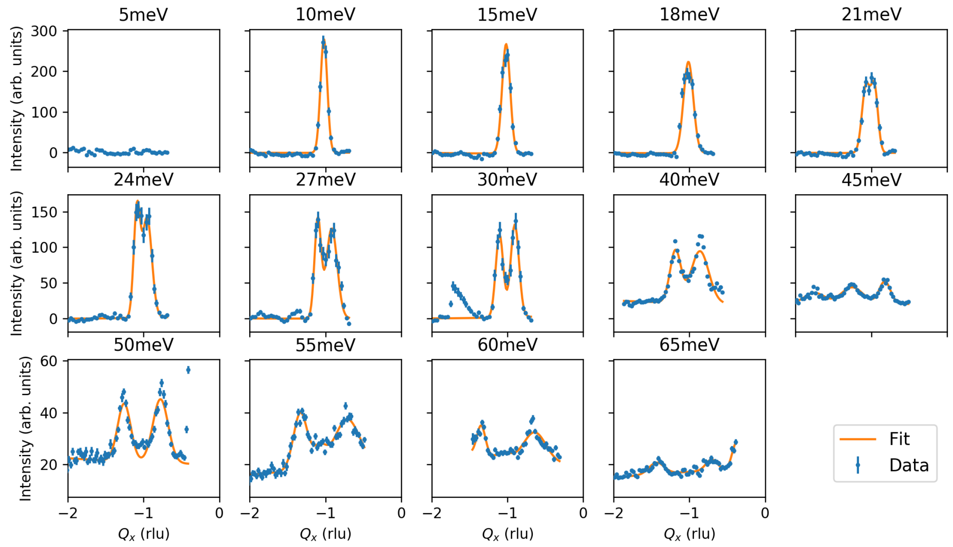


FIG. 3. One dimensional cuts along $\mathbf{Q} = (h01)$ of $h0l$ plane data for different $\Delta E$. Fits are shown in orange. To improve the signal to noise ratio at $\Delta E \geq 40$ meV, the integration was performed over specific detectors in the FlatCone array that did not intersect Al powder rings (whereas all detectors were utilised at low energies to construct these cuts).

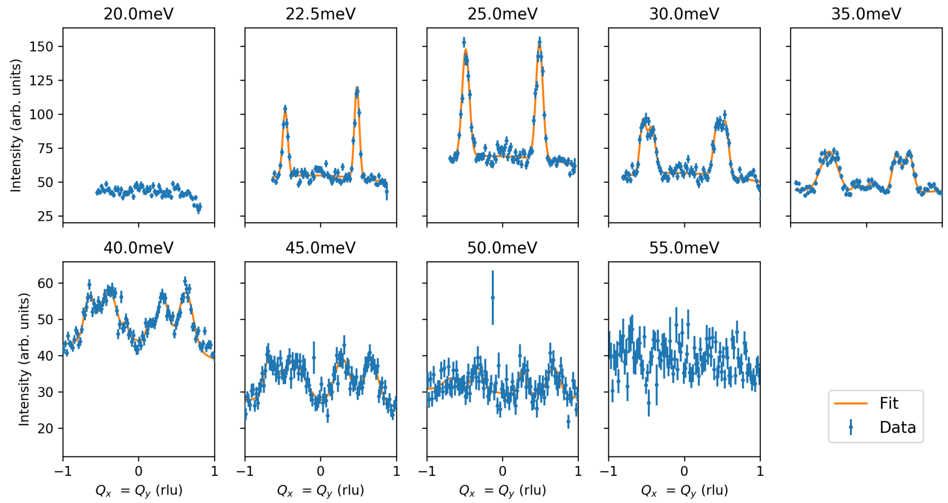


FIG. 4. One dimensional cuts along $\mathbf{Q} = (hh1)$ of $hhl$ plane data for different $\Delta E$. Fits are shown in orange. To improve the signal to noise ratio in the $hhl$ plane, the integration was performed over specific detectors in the FlatCone array that did not intersect Al powder rings.
